# Supplementary material for: Divide and Conquer Networks
Source: arXiv:1611.02401 source file (2018-10-14)
Supplement: Supplementary file 1 [file supplementary.tex]

\documentclass{article}

% if you need to pass options to natbib, use, e.g.:
% \PassOptionsToPackage{numbers, compress}{natbib}
% before loading nips_2017
%
% to avoid loading the natbib package, add option nonatbib:
% \usepackage[nonatbib]{nips_2017}

\usepackage{iclr2016_conference,times}

% to compile a camera-ready version, add the [final] option, e.g.:
% \usepackage[final]{nips_2017}

\usepackage[utf8]{inputenc} % allow utf-8 input
\usepackage[T1]{fontenc}    % use 8-bit T1 fonts
\usepackage{hyperref}       % hyperlinks
\usepackage{url}            % simple URL typesetting
\usepackage{booktabs}       % professional-quality tables
\usepackage{amsfonts}       % blackboard math symbols
\usepackage{nicefrac}       % compact symbols for 1/2, etc.
\usepackage{microtype}      % microtypography
\usepackage{amssymb,graphicx} % for math
\usepackage{amsmath}

\title{Supplementary Material for Divide and Conquer Networks}

% The \author macro works with any number of authors. There are two
% commands used to separate the names and addresses of multiple
% authors: \And and \AND.
%
% Using \And between authors leaves it to LaTeX to determine where to
% break the lines. Using \AND forces a line break at that point. So,
% if LaTeX puts 3 of 4 authors names on the first line, and the last
% on the second line, try using \AND instead of \And before the third
% author name.

\author{
  Alex Nowak \\
  Courant Institute of Mathematical Sciences\\
  Center for Data Science \\
  New York University\\
  New York, NY 10012, USA \\
  \texttt{alexnowakvila@gmail.com} \\
  %% examples of more authors
  \And
  Joan Bruna \\
  Courant Institute of Mathematical Sciences \\
  Center for Data Science \\
  New York, NY 10012, USA \\
  \texttt{bruna@cims.nyu.edu} \\
  %% \AND
  %% Coauthor \\
  %% Affiliation \\
  %% Address \\
  %% \texttt{email} \\
  %% \And
  %% Coauthor \\
  %% Affiliation \\
  %% Address \\
  %% \texttt{email} \\
  %% \And
  %% Coauthor \\
  %% Affiliation \\
  %% Address \\
  %% \texttt{email} \\
}

\begin{document}
% \nipsfinalcopy is no longer used

\maketitle

% \input{introduction}
% \input{relatedwork}
% \input{setup}
% \input{model}
% \input{training}
% \input{experiments}

% \input{conclusions}

% %\bibliography{biblio}

% \bibliography{mainbib}
% \bibliographystyle{plain} 

\appendix
\input{trainingapp}
\newpage
\input{kmeansapp}
\newpage
\input{convexhullapp}

\end{document}
